# Supplementary material for: Analyzing Intentional Behavior in Autonomous Agents under Uncertainty
Source: arXiv:2307.01532 source file (2023-07-04)
Supplement: Supplementary file 1 [file appendix.tex]

\section{Technical Appendix: Case-Study }
In this section we extend on the description of the environment used for our experiments that is briefly described in Section 6.1.

\begin{figure}[b]
    \centering
    \includegraphics[width=\linewidth]{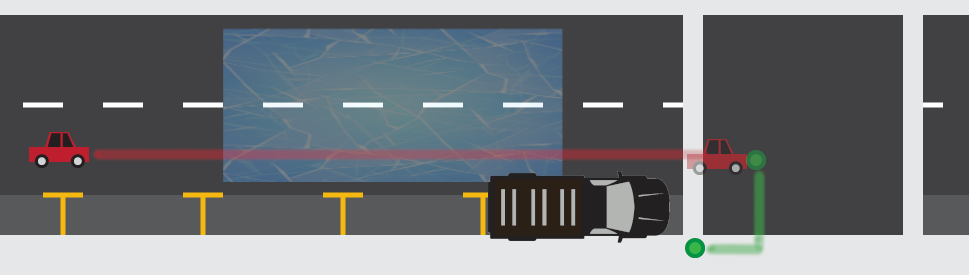}
    \caption{Case-study environment, with scenario $\tau_{\mathrm{ref}}$ highlighted.}
    \label{fig:casestudysettingappendix}
\end{figure}

\subsection{Dimensions and parts of the scenario}
The scenario, as depicted in Fig.~\ref{fig:casestudysettingappendix}, 
represents a two-way road, with parking spaces,
a sidewalk to the side, 
and a crosswalk in the right-most part.
The road contains a car (controlled by the agent under study) and
a pedestrian (green dot, modeled stochastically as part of the environment).
Other static elements may be other vehicles parked in the parking spaces available, 
that act blocking the visibility between the car and the pedestrian.
Another element affecting the scenario is that there is a patch of the road 
that is slippery due to adverse weather conditions.

We represent positions in the road as tuples $(x,y)$,
where $x$ represents the horizontal position and $y$ the vertical position.

The road length is $60$ m and the road width is $15$ m. The sidewalk has a width of $2$ m on one side and $1$ m on the other. The crosswalk has a width of $10$ m, 
and is located between $x_{cross}^{init} = 45$ m and 
$x_{cross}^{end} = 55$ m.
Concretely, any point $(x,y)$ with $y\in [0$ m$,2$ m$]\cup [14\mbox{ m},15\mbox{ m}]$ is on the sidewalk, 
and any point $(x,y)$ with $x\in[x_{cross}^{init}, x_{cross}^{end}]$ and not on the sidewalk is on the crosswalk. 
We say that the points with $x\in[x_{cross}^{init}, x_{cross}^{end}]$ and on the sidewalk 
are \emph{in front of the crosswalk}.
In the example we consider in this paper, as depicted in Fig.~\ref{fig:casestudysettingappendix}, 
there is a parked vehicle that can limit the car's vision of the pedestrian.
The coordinates of the bottom-left point of the vehicle are $(34\mbox{ m},2\mbox{ m})$, and the vehicle has a width of $2$ m and a lenght of $10$ m.

\subsection{Model of the car}
The car is modeled by its horizontal and vertical positions, 
represented by $x_c, y_c$ and its velocity $v_c$.
At each state, and depending on the action, the velocity increases by $\Delta v_c$.
In Table~\ref{tab:probabilitiesnormal} we specify the probabilities for each action and value of $\Delta v_c$. 
For example, when accelerating, the car increases velocity by $\Delta v_c = 1$ m/s with probability $0.5$, and increases velocity by $\Delta v_c =2$ m/s with probability $0.5$.

In all cases, the velocity is clipped to its corresponding range
between $v_{\min} = 0$ m/s and $v_{\max} = 5$ m/s.
Therefore the velocity update is given by:
\[
v_c^{new} = \max(v_{\min}, \min(v_{\max}, v_c^{old} + \Delta v_c )).
\]

The position $x_c$ is updated assuming a uniform motion at velocity $v_c^{new}$ 
for the space of $\Delta t = 1$ s, clipped to the range between 
$x_{\min} = 0$ and $x_{\max} = 60$.
The update is given by:
\[
x_c^{new} = \min(x_{\max}, x_c^{old} + v_c^{new}).
\]
The vertical position $y_c$ of the car does not change within a trace, 
since we do not consider wheel-steering moves. 
Therefore, it is not affected by any transition.

\paragraph{Effect of slippery road.}
The slippery range $[sl_{\mathrm{init}}, sl_{\mathrm{end}}]$ and 
the slippery factor $sl_{\mathrm{fact}}$ control the effect of road slipperiness
on the transition probabilities. 

The slippery range describes the range in the horizontal variable 
where slippery transitions apply. 
That is, whenever $x_c^{old}\notin [sl_{\mathrm{init}}, sl_{\mathrm{end}}]$, 
the regular transitions,
as given in Table~\ref{tab:probabilitiesnormal}, apply.
Otherwise, the transition probabilities used are the ones described in
the following paragraph. 

When the road is slippery, 
\ie, $c_x^{old}\in [sl_{\mathrm{init}}, sl_{\mathrm{end}}]$, 
the transition probabilities are those given in Table~\ref{tab:probabilitiesslippery},
where
\begin{gather}
\gamma_2 = 0.5/(2^{sl_{\mathrm{fact}}}-1), \qquad
\gamma_1 = 0.5/(2\cdot sl_{\mathrm{fact}}-1),\nonumber\\
\gamma_0 = 1 - \gamma_1 - \gamma_2.
\label{eqn:gamma}
\end{gather}
The rationale behind these transitions is to recover Table~\ref{tab:probabilitiesnormal} when $sl_{\mathrm{fact}} = 1$, 
and for larger values of the slippery factor, 
decrease the probability of changing speed.
Therefore, as the slippery factor grows, 
the change of speed by $\Delta v_c = 2$ m/s  
(both in acceleration and brake) 
becomes less likely than the change of speed by $\Delta v_c = 1$ m/s,
which in turn becomes less likely than just not changing speed,
\ie $\Delta v_c = 0$.
The remainder of the probability goes to $\Delta v_c = 0$ m/s. 
To provide the reader with some intuition about the numerical effect of the slippery factor, 
for $sl_{\mathrm{fact}} = 2.5$, 
we have $\gamma_0 \approx 0.77$,  $\gamma_1 \approx 0.12$, and $\gamma_2 \approx 0.11$.
On the extreme case of $sl_{\mathrm{fact}} = 4$, 
which is the limit in $sl_{\mathrm{fact}} = 4$ that we consider
for generating counterfactual scenarios,
we have $\gamma_0 \approx 0.9$, $\gamma_1 \approx 0.07$, and $\gamma_2 \approx 0.03$.

\begin{table}[t]
\begin{tabular}{llllll}
$\Delta v_c$ (m/s)           & -2  & -1  & 0   & +1  & +2  \\ \hline
accelerate & 0   & 0   & 0   & 0.5 & 0.5 \\
coast      & 0   & 0.1 & 0.9 & 0   & 0   \\
brake      & 0.5 & 0.5 & 0   & 0   & 0  
\end{tabular}
\caption{Transition probabilities for the car model for different actions and velocity updates.}
\label{tab:probabilitiesnormal}
\end{table}

\begin{table}[t]
\begin{tabular}{llllll}
$\Delta v_c$ (m/s)          & -2  & -1  & 0   & +1  & +2  \\ \hline
accelerate & 0   & 0   & $\gamma_0$   & $\gamma_1$ & $\gamma_2$ \\
coast      & 0   & 0.1 & 0.9 & 0   & 0   \\
brake      & $\gamma_2$ & $\gamma_1$ & $\gamma_0$   & 0   & 0  
\end{tabular}
\caption{Transition probabilities for the car model in the slippery part of the road, considering a slippery factor of $sl_{\mathrm{fact}}$.
The values of $\gamma_0,\gamma_1,\gamma_2$ are described in Equation~\ref{eqn:gamma}.}
\label{tab:probabilitiesslippery}
\end{table}

\paragraph{Effect of visibility block.}
At each state, whenever the line between the car front point and the pedestrian is blocked by 
any parked vehicle, we say that the visibility is blocked, meaning that the car cannot see the pedestrian. 

This affects the information available to the agent:
in states where the visibility line is not blocked, 
the agent has access to the position $(x_p, y_p)$ of the pedestrian.
Otherwise, the agent does not have that information, and thus 
no policy can use it to decide what to do with 

\subsection{Model of the pedestrian.}

The pedestrian is modeled by its horizontal and vertical positions
$x_p$ and $y_p$.
At each state, the pedestrian can move $+1$ m in any direction, or not move at all. 
The position of the pedestrian is updated with a position difference of $\Delta(x_p,y_p)$ as:
\[
\left(x_p^{new}, y_p^{new}\right) = \left(x_p^{new}, y_p^{new}\right) + \Delta\left(x_p,y_p\right),
\]
with the corresponding clipping of the positions to the ranges $[x_{\min}, x_{\max}]$, $[y_{\min}, y_{\max}]$,
that we omitted in the previous equation for the sake of avoiding unnecessary verbosity.

The pedestrian has three move regimes, that depend on the position of the pedestrian 
with respect to the crosswalk and the road, 
and that lead to different transition probabilities. 
In the following we describe the positions corresponding to the three regimes
and give a high level interpretation of the behavior of the pedestrian in each regime. 
The concrete probabilities for each value of $\Delta (x_p, y_p)$ at each regime are given in Table~\ref{tab:probabilitiespednormal}.
The three regimes are:
\begin{itemize}
    \item \emph{On the road.} When the pedestrian is not on the sidewalk, they will try to cross to the other side of the road.
    \item \emph{In front of the crosswalk.} When the pedestrian is on the sidewalk, in front of the crosswalk, 
    they will try in general to start crossing the street.
    \item \emph{On the sidewalk.} When the pedestrian is on the sidewalk but not in front of the crosswalk, 
    they will try in general to move in the direction of the crosswalk.
\end{itemize}

\paragraph{Effect of hesitancy.}

The values given in Table~\ref{tab:probabilitiespednormal} 
model a pedestrian that only cares about their own position
when deciding how to move, 
\ie whether they are on the road, on the sidewalk or in front of the crosswalk. 
A more reasonable pedestrian would modify their behavior in the
on-the-road regime to make sure that the chance of being hit by the car is low enough. 
To this end, we define the hesitancy factor $h_{\mathrm{fact}}$,
affecting the transition probabilities of the pedestrian when they
are on the road.

With the hesitancy factor active, 
we consider two sub-regimes of the on-the-road regime:
\begin{itemize}
    \item \emph{Danger to cross.} When the car is close to the pedestrian in the $x$ dimension, and
    the pedestrian would be at hitting position if they move vertically.
    In this case, a hesitant pedestrian favors staying at their position.
    \item \emph{Danger to stay.} When the car is close to the pedestrian in the $x$ dimension, and the pedestrian is already at hitting position. 
    In this case, a hesitant pedestrian favors moving vertically, 
    to exit as fast as possible the dangerous $y_p$ positions.
\end{itemize}

The concrete values of the transition probabilities are given in 
Table~\ref{tab:probabilitiespedhesitant}.
As can be deducted from the transitions in the table, 
the hesitancy factor is a number between 0 and 1.
A value of  $h_{\mathrm{fact}} = 1$ 
reduces the move of the pedestrian to the values in Table~\ref{tab:probabilitiespednormal}, 
and corresponds to a pedestrian that completely disregards the position of the car. 
A value of $h_{\mathrm{fact}} = 0$
completely blocks the pedestrian from putting themselves in a risky situation. 
We leave these two extreme cases outside of our counterfactual generation scheme. 

\begin{table}[t]
\begin{tabular}{llllll}
$\Delta (x_p, y_p)$ (m)          &  (+1,0)  & (0,+1)  & (0,0)  \\ \hline
On the road    & 0   & 0.7 & 0.3 \\
In front of crosswalk       & 0.45 & 0.45   & 0.1   \\
On the sidewalk      & 0.8   & 0.1   & 0.1  
\end{tabular}
\caption{Transition probabilities of the pedestrian for different regimes and updates.}
\label{tab:probabilitiespednormal}
\end{table}

\begin{table}[t]
\begin{tabular}{llllll}
$\Delta (x_p, y_p)$ (m)          &  (+1,0)  & (0,+1)  & (0,0)  \\ \hline
Danger to cross    & 0   & $1-0.3\cdot h_{\mathrm{fact}}$ & $0.3\cdot h_{\mathrm{fact}}$ \\
Danger to stay       & 0 & $0.7\cdot h_{\mathrm{fact}}$   & $1-0.7\cdot h_{\mathrm{fact}}$    \\
No danger      & 0   & 0.7   & 0.3  
\end{tabular}
\caption{Transition probabilities for the pedestrian sub-regimes of the on-the-road regimes, considering a hesitancy factor $h_{\mathrm{fact}}$.}
\label{tab:probabilitiespedhesitant}
\end{table}

\subsection{Special transitions.}
There are two cases in which the MDP transitions to a special sink state $s_{\mathrm{end}}$. 
This can be though as an ``end execution'' state,
as it is a state that transitions to itself with probability 1. 
A trace $\tau = (s_1, \dots, s_n)$ can end in the sink state $s_n = s_{\mathrm{end}}$ in three cases:
\begin{itemize}
    \item \emph{Car reaches end of street.} When $x_c = x_{\max}$, 
    it means that the car has reached the end of the street without 
    hitting the pedestrian. 
    \item \emph{Crash.} Whenever there is a collision between the car and the pedestrian.
\end{itemize}
